# Supplementary material for: ActiveCheerios: 3D-Printed Marangoni-Driven Active Particles at an Interface
Source: arXiv:2411.16011 source file (2024-11-24)
Supplement: Supplementary file 1 [file SI.tex]

% %\documentclass[10.75pt, a4paper]{article}
% %\input{initialisation.tex}

% %\begin{document}


% %%% SUPPPLEMENTARY INFORMATION %%%

% \section*{Supporting Information for}

% \textbf{Title: }Fragmentation and aggregation of cyanobacterial colonies
% \\
% \textbf{Authors: }Yuri Z. Sinzato, Robert Uittenbogaard, Petra M. Visser, Jef Huisman and Maziyar Jalaal
% \\
% \textbf{Corresponding authors: }Maziyar Jalaal (m.jalaal@uva.nl) / Yuri Z. Sinzato (y.z.sinzato@uva.nl)


% \clearpage
% \section*{Supporting Information Text}

% \subsection*{Field sample collection}

% Samples of \textit{Microcystis} spp. were collected from Lake Gaasperplas - the Netherlands - at the sampling point 52°18'31.0"N 4°59'59.2"E on 14th August 2022, at 14:00. This is an artificial lake used for recreational purposes. No visible surface scums were present at the time of sampling. Water quality measurements of Lake Gaasperplas were obtained from the \href{https://www.waterkwaliteitsportaal.nl/oppervlaktewaterkwaliteit}{Dutch Water Authority (Rijkswaterstaat)}. Figure \ref{fig:field_samples} shows micrographic images of the phytoplankton samples. 

% \subsection*{Image analysis}

% This section describes the routine used to analyze raw images of the aggregation and fragmentation process of \textit{Microcystis} colonies under a cone-and-plate shear setup. Each frame has dimensions of 2048x2048 pixels. Prior to each experiment, $3.5$ ml of distilled water was pipette in the setup, and 200 frames were captured at $\dot{\varepsilon} = 0.019$ ${m^2/s^3}$ and 10 fps. A background image was generated by averaging over the frames and applying a Gaussian blur filter. After that, the distilled water was discarded, and $3.5$ ml of cyanobacteria suspension was pipetted into the setup. Each time point in the data sets corresponds to a stack of 200 frames. Two treatments are made, one to detect small colonies(or single cells) and another to detect large colonies:
% \begin{itemize}
%     \item Small colonies ($l<5$): Image is cropped into a smaller section (500x500 pixels), to speed the processing. The background is subtracted using the reference image. The image intensity is renormalized and then thresholded. Small features ($0.5<l<5$) are segmented, measured, and counted.
%     \item Large colonies ($l>5$): A Gaussian blur is applied to filter small colonies. The background is subtracted using a reference image. The image intensity is renormalized and then thresholded. Small features ($l>5$) are segmented, measured, and counted.
% \end{itemize}
% For each time point, the counted features of the 200 frames were distributed in bins of width $\Delta l = 0.5$. Since not all colonies are within the depth-of-focus, a correction function for the featured count was estimated using a suspension with a known size distribution, given by:
% \begin{eqnarray}
% N_c[i] =
%     \begin{cases}
%          (\lambda_3 + \lambda_1\, (\lambda_2 - \lambda_3))\, N_p[i] &, ~ \text{if } l[i] \leq 2 \\
%         (\lambda_3 + \lambda_1\, (\lambda_2 - \lambda_3)(4-l[i])/2)\, N_p[i]  &, ~ \text{if } 2 < l[i] \leq 4 \\
%         \lambda_3\, N_p[i] &, ~ \text{if } 4 < l[i] \leq 5 \\
%         \lambda_4\, N_p[i] &, ~ \text{if } l[i] > 5
%     \end{cases}
% \end{eqnarray}
% Here, $N_p[i]$ and $N_c[i]$ are the number of features before and after correction in a bin centered at $l[i]$. To obtain the calibration parameters $\lambda_i$, a sample of filtered colonies of \textit{Microcystis} strain V163 was subjected to the cone-and-plate shear setup for 2 min at $\dot{\varepsilon} = 0.019$ ${m^2/s^3}$, and then transferred to a counting chamber. The latter was used as a standard for the size distribution. The calculated parameters were $\lambda_1 = 1$, $\lambda_2 = 73.13$, $\lambda_3 = 13.71$ and $\lambda_4 = 1.24$. The small size range ($l \leq 4$) has low precision due to the pixel resolution, therefore the parameter $\lambda_1$ was adjusted to ensure biovolume conservation. The value of $\lambda=1$ was used for $t=0$, and it was fitted in each subsequent time point so that the total cell count is constant through time. Finally, the normalized biovolume distribution for each time point is calculated.

% For the direct computation of the fragmentation frequency, a pure fragmentation with an ideal binary erosion was assumed, such that the time derivative of the colony size distribution is
% \begin{equation}
%     \dfrac{\mathrm{d}}{\mathrm{d}t}N_p[i](t) = - \dfrac{\kappa[i] \, N_p[i](t)}{l^f[i] - l^f[i-1]} + \dfrac{\kappa[i+1] \, N_p[i+1](t)}{l^f[i+1] - l^f[i]}~, 
%     \label{eq:Kb_calcSI}
% \end{equation}
% where $N_p[i](t)$, $\kappa[i]$, and $l[i]$ refer to the bin count, fragmentation frequency, and relative diameter at the center of bin $i$. This formula is only valid for the bins larger than the single cell, as the latter does not suffer fragmentation. The bin count distribution $N_p[i]$ is initialized with the experimental value, and an initial guess fragmentation frequency $\kappa[i]$ is made for all bins larger than a single cell. The values of $N_p[i]$ are evolved in time using the Python solver {\tt scipy.integrate.solve\_ivp}, with an implicit Radau method. For each bin, the cumulative squared error between the experimental and numerical bin counts is computed. The error is minimized using the values of $\kappa[i]$ as the optimization parameter and the Python solver {\tt scipy.optimize.minimize}. The uncertainty of $\kappa[i]$ is propagated from \eqref{eq:Kb_calcSI} talking into account the bin count uncertainty. The bin size for each dataset was chosen in order to minimize the bin count uncertainty. The script for image analysis is available \href{https://github.com/FluidLab/CyanoB_Agg_Frag.git}{here}.

%  \subsection*{Fragmentation measurements with \textit{Microcystis} strain V163}

% Additional measurements of fragmentation of large colonies of \textit{Microcystis} strain V163 were performed. Colonies grown by cell division were filtered through a mesh of $53~\mu m$, and the collected colonies were redispersed in BG-11 medium. Under moderate dissipation rate of $\dot{\varepsilon} = 0.019~ {m^/s^3}$ the fragmentation was negligible (Fig. \ref{fig:frag_extra_1}), with the median size and fraction of large colonies remaining stable over 5 hours of flow. The behavior is independent of the total biovolume fraction, showing that aggregation rates are negligible for large colonies. In contrast, the steady median size for small colonies increases with the total biovolume fraction, although still an order of magnitude smaller than division-formed colonies. Significant fragmentation can be seen from a dissipation rate of $\dot{\varepsilon} = 5.8~ {m^/s^3}$ (Fig. \ref{fig:frag_extra_2}). For a large value of $\dot{\varepsilon} = 9.6~ {m^/s^3}$, the small colonies become the largest fraction in below $5$ min (the smallest time resolution in our setup). 

%  \subsection*{Aggregation measurements with \textit{Microcystis} strain V163}

% Additional measurements of aggregation of single cells of \textit{Microcystis} strain V163 were performed. The suspension was filtered through a $25~\mu m$ filter paper to select mostly single cells. Under moderate dissipation rate of $\dot{\varepsilon} = 0.019~ {m^/s^3}$, the aggregation increased with the total biovolume fraction $\phi$ (Fig. \ref{fig:agg_extra}). Under an intense dissipation rate of $\dot{\varepsilon} = 5.8~ {m^/s^3}$, no aggregation was observed, and the median size of colonies remained equal to the initial value (near the single-cell size).


% \subsection*{Rate of increase in the average colony size due to pure aggregation}

% Consider a suspension of colonies subjected only to aggregation, neglecting cell division and fragmentation. In this case, the time derivative of the normalized biovolume distribution $n(l,t)$ is given by \cite{burd2009particle}: 
% \begin{eqnarray}
% 	\dfrac{\partial}{\partial t}n(l,t)= \dfrac{6\, \phi \, \alpha}{\pi} \left[ \dfrac{1}{2} \int_{0}^{l} \beta(l',l_o) \left(\dfrac{l}{l' l_o}\right)^{2f -1 } n(l',t)\, n(l_o,t)\, \mathrm{d}l'  \right. \nonumber\\ 
% 	\left.  -  n(l,t)\int_{0}^{\infty} \beta(l,l')\,  \dfrac{1}{l'^{f}}\, n(l',t)\, \mathrm{d}l' \right] ~,
% 	\label{eq:dndt_agg_SI}
% \end{eqnarray}
% where $l_o = (l^{f} - l'^{f})^{1/f}$, and the collision frequency kernel is $\beta(l,l')$. The average colony size is defined as $\overline{l} = \int_0^{\infty}l \, n(l,t)\mathrm{d}l$. Applying this definition to Eq. \eqref{eq:dndt_agg_SI}, we obtain that the time derivate of $\overline{l}(t)$ follows:
% \begin{eqnarray}
% 	\dfrac{\partial}{\partial t}\overline{l}(t)= \dfrac{6\, \phi \, \alpha}{\pi} \left[ \dfrac{1}{2} \int_{0}^{\infty} \int_{0}^{l} \beta(l',l_o)\,  l \, \left(\dfrac{l}{l'\,  l_o}\right)^{2f -1 } n(l',t)\, n(l_o,t)\, \mathrm{d}l'\mathrm{d}l  \right. \nonumber\\ 
% 	\left.  -  \int_{0}^{\infty} \int_{0}^{\infty} n(l,t)\,  \beta(l,l') \, l\,  \dfrac{1}{l'^{f}}n(l',t)\, \mathrm{d}l'\mathrm{d}l \right] ~.
% 	\label{eq:dldt_agg_SI}
% \end{eqnarray}
% If we assume that the size distribution remains monodisperse for short times, we can write that $n(l,t) = \delta(l - \overline{l}(t))$. Substituting this hypothesis into Eq. \eqref{eq:dldt_agg_SI} results that
% \begin{eqnarray}
% 	\dfrac{\partial}{\partial t}\overline{l}(t)= \dfrac{6\, \phi \, \alpha}{\pi} \left[ \dfrac{1}{2} \int_{0}^{\infty} \int_{0}^{l} \beta(l',l_o)\,  l \, \left(\dfrac{l}{l' l_o}\right)^{2f -1 } \delta(l' - \overline{l})\, \delta(l_o - \overline{l})\, \mathrm{d}l'\mathrm{d}l  \right. \nonumber\\ 
% 	\left.  -  \int_{0}^{\infty} \int_{0}^{\infty} \delta(l - \overline{l})\,  \beta(l,l') \, l \, \dfrac{1}{l'^{f}}\, \delta(l' - \overline{l})\, \mathrm{d}l'\mathrm{d}l \right] ~.
% 	\label{eq:dldt_agg_2SI}
% \end{eqnarray}
% Applying a variable change, the integral can be rewritten as:
% \begin{eqnarray}
% 	\dfrac{\partial}{\partial t}\overline{l}(t)= \dfrac{6\, \phi\,  \alpha}{\pi} \left[ \dfrac{1}{2} \int_{0}^{\infty} \int_{0}^{\infty} \beta(l',l_o)\,  l \, \left(\dfrac{l}{l' l_o}\right)^{2f -1 } \, \delta(l' - \overline{l})\, \delta(l_o - \overline{l})\, l_o^{f-1}\, (l_o^f + l'^f)^{\frac{1}{f}-1} \, \mathrm{d}l_o\mathrm{d}l'  \right. \nonumber\\ 
% 	\left.  -  \int_{0}^{\infty} \int_{0}^{\infty} \delta(l - \overline{l}) \, \beta(l,l') \, l \, \dfrac{1}{l'^{f}}\, \delta(l' - \overline{l})\, \mathrm{d}l'\mathrm{d}l \right] ~.
% 	\label{eq:dldt_agg_3SI}
% \end{eqnarray}
% Solving the integral and applying the model for the collision kernel in a turbulent shear flow \cite{saffman1956collision}, $\beta(l,l')=0.163\,(l+l')^3\,\sqrt{\dot{\varepsilon}/\nu}$, results that the rate of increase in the average colony size is:
% \begin{eqnarray}
% 	\dfrac{1}{\overline{l}} \dfrac{\mathrm{d}\overline{l}}{\mathrm{d}t} = 2.49\, (\sqrt[f]{2}-1)\, \phi \, \alpha\,  \overline{l}^{4-2f}\sqrt{\dfrac{\dot{\varepsilon}}{\nu}}~.
% 	\label{eq:dldt_agg_4SI}
% \end{eqnarray}
% In the limit of fractal dimension $f = 2$, the growth rate reduces to;
% \begin{eqnarray}
% 	\dfrac{1}{\overline{l}} \dfrac{\mathrm{d}\overline{l}}{\mathrm{d}t} = 1.03\,  \phi\,  \alpha\,  \sqrt{\dfrac{\dot{\varepsilon}}{\nu}}~,
% 	\label{eq:dldt_agg_5SI}
% \end{eqnarray}
% which is independent of $\overline{l}$.

%  \subsection*{Rheological characterization of concentrated colonies of \textit{Microcystis} strain V163}
% A steady-shear (Fig. \ref{fig:rheology}A) and a large-amplitude-oscillatory-shear (Fig. \ref{fig:rheology}B) tests were performed in a sample of concentrated colonies of \textit{Microcystis} strain V163. Due to the limited volume of samples available after separation, only one repetition was possible for each test. Before each test, the sample was subject to a pre-shear at $\dot{\gamma} = 10$ s$^{-1}$ for 200s, followed by 100s of rest. For the steady-shear test, the minimum transient time was determined in a separate test (40s for $\dot{\gamma} = 100$ s$^{-1}$  to 200s for $\dot{\gamma} = 0.001$ s$^{-1}$). For the oscillatory shear, the minimum transient time was determined by the rheometer software. A Herschel–Bulkley fit was applied to the steady shear data, $\tau = \tau_y + k\dot{\gamma}^n$, from which a dynamical yield stress $\tau_y = 4.3 \pm 0.3 \text{ Pa}$ (SD from best fit) was estimated.

% \subsection*{Comparison of hypothesis for the fragment distribution function}

% Assuming a binary fragmentation (\textit{i.e.,} two fragments per fragmentation event), the fragment size distribution can be written in the form $g_i(l,l') = \delta(l - l_a) + \delta(l - l_b)$, where $l_a$ and $l_b$ are the size of fragments. Two ideal models for binary fragmentation are erosion and equal fragments, described by the following functions:
% \begin{eqnarray}    
%     g(l,l') = \begin{cases}
%         \delta(l - 1) + \delta(l - \sqrt[f]{l'^{f} -1}) & \text{(Erosion),} \\
%         2 \delta(l - {l'/\sqrt[f]{2}}) & \text{(Equal fragments).}
%     \end{cases} 
% \end{eqnarray}
% Due to a lack of experimental evidence of single colony fragmentation events, both models were tested for the category $C_2$ colonies.  The equal fragments hypothesis was chosen as it better captures the experimental results for the size distribution of \textit{Microcystis} strain V163 colonies aggregated from single cells (Fig. \ref{fig:frag_hypo}).

% \subsection*{Cone-and-plate shear setup}

% The turbulent shear was generated by a cone-and-plate shear, with the dimensions depicted in Fig. \ref{fig:lam_turbulence}A. The flow regime can be identified from the average energy dissipation rate $\dot{\varepsilon}$ curve against the angular velocity $\omega$, with a $\sim \omega^2$ dependence in the laminar regime and a  $\sim \omega^{5/2}$ dependence in the inertial region (Fig. \ref{fig:lam_turbulence}B) \cite{sdougos1984secondary,grad2000spectral}. The Kolmogorov scale $\eta$, which is an estimate of the size of the smallest eddies in a turbulent flow, can be calculated from the relation $\eta = \nu^{3/4} \dot{\varepsilon}^{-1/4}$. The Kolmogorov scale in our results range from $\eta \sim 85 ~\mu$m for the lowest dissipation rate ($\dot{\varepsilon} = 0.019~{m^2/s^3}$) to $\eta \sim 18 ~\mu$m for the highest dissipation rate ($\dot{\varepsilon} = 9.6~{m^2/s^3}$).

% \printbibliography

% %%% Each figure should be on its own page

% \clearpage
% \begin{figure*}[h]
%     \centering
%     \includegraphics[width=17.8cm]{Figures/Figure S1 - Field samples microscopy.pdf}
%     \caption{(A-D) Micrographic images of phytoplankton field samples collected from the surface layer of Lake Gaasperplas. \textit{Microcystis} spp. are dominant in the sample.}
%     \label{fig:field_samples}
% \end{figure*}

% \clearpage
% \begin{figure*}[h]
%     \centering
%     \includegraphics{Figures/Figure S2 - Fragmentation extra 1 phi.pdf} 
%     \caption{Kinetics of the fragmentation of \textit{Microcystis} strain V163 colonies under a moderate dissipation rate ($\dot{\varepsilon} = 0.019~ {m^/s^3}$) and various values of total biovolume fraction. The laboratory culture was filtered to select mainly large colonies, and total biovolume fraction was adjusted. Plots in the left column depict the median diameter of each size population as a function of time, where bars and shaded regions indicate limits of 25th and 75th percentiles. Plots in the right column depict the fraction of small colonies as a function of time. The total biovolume fraction is (A-B) $\phi = 10^{-4}$, (C-D) $\phi = 2 \cdot 10^{-4}$, (E-D) $\phi = 5 \cdot 10^{-4}$. Best fit parameters: $\alpha_1 = 0.023$,  $S_1= 0.034$ , $q_1 = 4.5$, $S_2= 31$ , $q_2 = 4.1$.}
%     \label{fig:frag_extra_1}
% \end{figure*}

% \clearpage
% \begin{figure*}[h]
%     \centering
%     \includegraphics{Figures/Figure S3 - Fragmentation extra 2 eps.pdf} 
%     \caption{Kinetics of the fragmentation of strain V163 colonies under a moderate total biovolume fraction ($\phi = 10^{-4}$) and various values of dissipation rate. The laboratory culture was filtered to select mainly large colonies, and total biovolume fraction was adjusted. Plots in the left column depict the median diameter of each size population as a function of time, where bars and shaded regions indicate limits of 25th and 75th percentiles. Plots in the right column depict the fraction of small colonies as a function of time. The dissipation rate is (A-B) $\dot{\varepsilon} = 1.1~ {m^/s^3}$, (C-D) $\dot{\varepsilon} = 5.8~ {m^/s^3}$, (E-D) $\dot{\varepsilon} = 9.6~ {m^/s^3}$. Best fit parameters: $\alpha_1 = 0.023$,  $S_1= 0.034$ , $q_1 = 4.5$, $S_2= 31$ , $q_2 = 4.1$.}
%     \label{fig:frag_extra_2}
% \end{figure*}

% \clearpage
% \begin{figure*}[h]
%     \centering
%     \includegraphics{Figures/Figure S4 - Aggregation extra.pdf} 
%     \caption{Kinetics of the aggregation of \textit{Microcystis} strain V163 colonies under a moderate dissipation rate ($\dot{\varepsilon} = 0.019~ {m^/s^3}$) and various values of total biovolume fraction. The laboratory culture was filtered to select mostly single cells, and the total biovolume fraction was adjusted. Plots in the left column depict the median diameter of each size population as a function of time, where bars and shaded regions indicate limits of 25th and 75th percentiles. Plots in the right column depict the fraction of small colonies as a function of time. The total biovolume fraction is (A-B) $\phi = 10^{-4}$, (C-D) $\phi = 2 \cdot 10^{-4}$, (E-D) $\phi = 5 \cdot 10^{-4}$. Best fit parameters: $\alpha_1 = 0.023$,  $S_1= 0.034$ , $q_1 = 4.5$, $S_2= 31$ , $q_2 = 4.1$.}
%     \label{fig:agg_extra}
% \end{figure*}

% \clearpage
% \begin{figure*}[h]
%     \centering
%     \includegraphics{Figures/Figure S5 - Rheology.pdf} 
%     \caption{Rheology of concentrated colonies of \textit{Microcystis} strain V163. (A) Shear stress as a function of the shear rate obtained for a steady shear test. Solid line indicates a Herschel–Bulkley fit, $\tau = \tau_y + k\dot{\gamma}^n$, where $\tau_y = 4.3 \pm 0.3 \text{Pa}$ (SD from best fit) is the dynamical yield stress. Other fit parameters are $k = 0.55 \pm 0.13$ and
% $n = 0.85 \pm 0.05$  (B) Storage $G'$ and loss $G''$ moduli as a function of the deformation strain amplitude $\gamma$ for a oscillatory shear with angular frequency of $1 \text{ rad/s}$. }
%     \label{fig:rheology}
% \end{figure*}

% \clearpage
% \begin{figure*}[h]
%     \centering
%     \includegraphics{Figures/Figure S6 - Fragment hypothesis.pdf} 
%     \caption{Comparison of hypothesis for the fragment distribution of category $C_1$ colonies. Bars show the experimental results for normalized biovolume distribution of filtered single cells of \textit{Microcystis} strain V163 after 1 hour under a moderate dissipation rate ($\dot{\varepsilon} = 0.019~ {m^/s^3}$) and a total biovolume fraction of $\phi = 10^{-4}$. Lines depict the prediction of the sectional method using an equal fragment hypothesis (dashed) and an erosion hypothesis (solid).}
%     \label{fig:frag_hypo}
% \end{figure*}

% \clearpage
% \begin{figure*}[h]
%     \centering
%     \includegraphics[width=\textwidth]{Figures/Figure S7 - Cone and plate.pdf}
%     \caption{Cone-and-plate setup used to generate a turbulent shear in a suspension of \textit{Microcystis} colonies. (A) Schematics of the components with the main dimensions indicated in millimeters. (B) Average energy dissipation rate as a function of the angular velocity of the conical probe. Bullets indicate the measured data, and the solid lines indicate the best fit of the laminar regime ($\sim \omega^2$ ) and the inertial regime ($\sim \omega^{5/2}$).}
%     \label{fig:lam_turbulence}
% \end{figure*}

% %\end{document}
